# Supplementary material for: LLOL: Low-Latency Odometry for Spinning Lidars
Source: arXiv:2110.01725 source file (2022-04-13)
Supplement: Supplementary file 1 [file s70_appendix.tex]

\section*{Appendix}
